# Supplementary material for: Anisotropic anomalous diffusion in microgravity dusty plasma. Part One: Nonextensive Statistical Analysis
Source: arXiv:2411.15705 source file (2025-04-23)
Supplement: Supplementary file 1 [file appendix.tex]

\section{Appendix \centering}
\label{sec:Appendix}

Previous studies have shown that a kappa distribution, which is the same as a q-Gaussian distribution, could serve to fit, however here we look in more detail at how the underlying physics of the nonextensive parameter q behaves with cases of changes pressure and current. We also notice that the dusty plasma coupling parameter is proportional to potential energy over kinetic energy $\Gamma \propto \frac{PE}{KE}$. Connection between Order Parameter (maybe Coupling? $\Gamma_x=\frac{Q^2 e^{\frac{-a_x}{\lambda_Dx}}}{a_x k_B T_x }$, and q, since electrons are ‘sloshing’ back and forth so much mostly in x-direction $\lambda_Dx$ is large (assuming incorrect Debye potential as first order approximation)  making $\Gamma_x>1$ but y-direction $\Gamma_y<1$ so does $q \approx 1-\frac{1}{3/5-\Gamma}$  work as an expression)? Analysis on pair correlation function by Matthews et al. [] and the liquid-crystal behavior of PK-4 and how this relationship compares with the above.

\begin{table}[htbp!]
  \centering
  \captionsetup{labelsep=none}
  \begin{tabular}{|c|c|c|c|c|}
    \hline
    610.72 & 606.84 & 578.34 & 540.47 & 503.85 \\
    \hline
    599.40 & 574.31 & 562.82 & 539.52 & 480.10 \\
    \hline
    580.27 & 567.10 & 536.33 & 550.55 & 479.73 \\
    \hline
    599.48 & 560.61 & 520.86 & 528.10 & 485.26 \\
    \hline
  \end{tabular}
  \caption*{$v_{th\parallel}$}
  \label{4x5_zeroes}
\end{table}

\begin{table}[htbp!]
  \centering
  \captionsetup{labelsep=none}
  \begin{tabular}{|c|c|c|c|c|}
    \hline
    512.37 & 474.95 & 431.33 & 426.35 & 457.32 \\
    \hline
    489.23 & 471.62 & 441.13 & 459.42 & 408.58 \\
    \hline
    490.60 & 469.00 & 463.54 & 465.65 & 439.63 \\
    \hline
    422.57 & 346.65 & 329.65 & 301.60 & 379.21 \\
    \hline
  \end{tabular}
  \caption*{$v_{th\perp}$}
  \label{4x5_zeroes}
\end{table}
{\color{red} Luca: No caption? What do these tables contain and why are they here?}

Starting from the original theory by Einstein, an ensemble of particles undergoing Brownian motion will have the following density:

\begin{equation}
    f(r,t)=\frac{\rho_0}{\sqrt{4\pi Dt}}e^{-\frac{(r-r_0)^2}{4Dt}}
\end{equation}

assuming all the particles were followed from a single point at $t=0$, that $r$ is the distance to this point, and $D$ the diffusion coefficient. This also relates to the standard Boltzmann-Gibbs theory of thermodynamics. Using this formula, one can derive the mean square displacement (MSD) for this type of particle:

\begin{equation}
    \langle |r(t)-r_0|^2\rangle = \frac{1}{N}\sum_{i=1}^N |r^{(i)}(t)-r^{(i)}(0)|^2 = 2dDt
\end{equation}

where d is the dimensionality and D the diffusion coefficient. Then a mean is taken over a whole ensemble of particles: you have to sample many particles, compute $MSD_i (\tau)=(r_i (\tau)-r_i (0))^2$ for each particle i and average the resulting $MSD_i$ over all particles. It is also known that the Langevin equation for a Brownian particle is simply:

\begin{equation}
    \frac{d\boldsymbol{u}}{dt}=-\zeta \boldsymbol{u} +A(t)
\end{equation}
	
Where $\boldsymbol{u}$ is the velocity vector, $\eta$ is the friction coefficient divided by the mass, and $A(t)$ is a randomly varying vector function. A particle with this stochastic differential equation is known to have the following relation with the $MSD$:

\begin{equation}
    \begin{aligned}
        \langle |r-r_0|^2\rangle \to |u_0|^2t^2 \text{ when } t \to 0 \\
        \langle |r-r_0|^2\rangle \to \frac{6k_BT}{m\zeta}t \text{ when } t >> 0
    \end{aligned}
\end{equation}

This is the original theory developed to understand and describe particle diffusion.

Also recall the linear Fokker-Planck equation and remove drift, which removing constant $K$ from the equation and potential $U$ from the solution. 

\begin{equation}
    \frac{\partial p(x,t)}{\partial t}=D \frac{\partial^2 p(x,t))}{\partial x^2}
\end{equation}
{\color{red} Luca: Is this equation there by itself? Don't make an equation into a sentence.}
Non-extensive entropic systems developed by Tsallis, is a generalization of the Boltzmann Entropy expressed with a q logarithm $S_q=kln_q(\Omega)=k\frac{1-\sum_{i=1}p_i^q}{q-1}$. This entropy is nonadditive when $q\neq 1$ meaning $S_q (A+B)\neq S_q (A)+S_q$ (B) rather $S_q (A+B) = S_q (A)+S_q (B)+(1-q) S_q (A) S_q (B)$ and therefore in the case $q>1$ this system is called subadditive $S_q (A+B)\leq S_q (A)+S_q (B)$. The motivation of this theory stems from the fact that the thermodynamic limit within Boltzmann statistics does not seem to work in a system of particles interacting via long-range forces, which makes the statistical description of plasmas challenging. This is especially challenging for low temperature plasmas or complex plasmas such as a dusty plasma. Consider integrating a potential of the form $U(r)=-\frac{A}{r^\xi}  (A>0 ; \xi \geq 0)$ and finding the total potential energy per $N$ number of particles $U(N)/N \propto A \int_{1}^{N^{\frac{1}{d}}}\frac{1}{r^\xi}r^{d-1}dr$ then in the limit as you move form the micro to meso or macroscopic your particles $N\to \infty$ therefore:

\begin{equation}
    \lim_{N\to \infty} \frac{U(N)}{N} \to
    \begin{cases}
        -\frac{A}{\xi -d} & \text{if } \frac{\xi}{d}>1 \\ ln(N)\to \infty & \text{if } \frac{\xi}{d}=1 \\
        \frac{N^{1-\frac{\xi}{d}}}{1-\frac{\xi}{d}}\to \infty & \text{if } 0<\frac{\xi}{d}<1
    \end{cases}
\end{equation}

The term $\frac{\xi}{d}$ is the microscropic ratio and is greater than 1 for short range potentials such as the Lenard-Jones $(\xi=6)$ in $3-D$ space. Also, in the case where $\frac{\xi}{d}>1$, the potential still depends on the dimension $d$ and is therefore extensive. However, for the long-range case $0<\frac{\xi}{d}<1$ the potential we tried per $N$ particles blows up to infinity therefore it does not seem to depend on the system size and would be nonextensive. To better understand this consider a large system $\Sigma$ with $U(\Sigma)$ being the potential energy of $\Sigma$. If we try to calculate for a large system $\lambda\Sigma$, with $\lambda$ being a scaling parameter $(\lambda>1)$, and using the fact that the number of particles are extensive $N(\lambda\Sigma)=\lambda N(\Sigma)$ then for $N>>1$ we get:

\begin{equation}
    \frac{U(\lambda\Sigma}{U(\Sigma)}=\lambda \frac{(\lambda N)^{1-\frac{\xi}{d}}-1}{(N)^{1-\frac{\xi}{d}}-1} \approx
    \begin{cases}
        \lambda & \text{if } \frac{\xi}{d}\geq1 \\
        \lambda^{2-\frac{\xi}{d}} & \text{if } 0<\frac{\xi}{d}<1
    \end{cases}
\end{equation}

The result does not depend on the microscopic ratio $\frac{\xi}{d}$ for short-range interactions, but it does for long-range interactions. Therefore, we want to generalize the Boltzmann-Gibbs Entropy $S_{BG}$ so that no matter the range of interaction it preserves its extensivity. That is the purpose to which Tsallis created his entropy equations, now called Tsallis entropy.

Lastly, Fig. \ref{fig:alphavtau} shows how $\alpha$ changes as a function of time delay $\tau$.

\begin{figure}[H] 
    \centering
    \includegraphics[width=120mm,height=50mm]{Photos/alpha vs tau.png}
    \caption{Plot of calculated $\alpha$ from q position distributions at different delays on left and plot of $\alpha$ from MSD fits at different delays on right.}
    \label{fig:alphavtau}
\end{figure}

The plot of $q$ vs. $\tau$ shows a clear decaying increase that is approximately $(5/3 \pm \delta -e^{-\tau}$) to some steady-state value of q while something similar may be happening in the $\alpha$ vs. $\tau$ case, it is hard to say since the error on the MSD plots grows large after $\tau > 10$. {\color{red} Luca: Run-on sentence.} This would seemingly mean there is a maximum degree of anomalous diffusion at large time delay intervals.

\end{document}
